# Supplementary material for: Genetic networks with canalyzing Boolean rules are always stable
Source: arXiv:q-bio/0412005 source file (2004-12-02)
Supplement: Supplementary file 1 [file suppl.pdf]

## Supporting Text

**Approximation of the Multinomial.** Using Stirling's approximation

$$n! \approx (n/e)^n \sqrt{2\pi n}\ , \qquad \textbf{[S1]}$$

we get

$$\binom{N}{\mathbf{n}} \approx \frac{N^N\sqrt{2\pi N}}{\prod\limits_{\substack{0\le i<m\\ n_i\neq 0}} n_i^{n_i}\sqrt{2\pi n_i}}\ . \qquad \textbf{[S2]}$$

The right hand side in Eq. **S2** is an upper bound to the multinomial. To show this, we take advantage of the inequality

$$e^{1/(12n+1)}(n/e)^n\sqrt{2\pi n} < n! < e^{1/(12n)}(n/e)^n\sqrt{2\pi n} \qquad \textbf{[S3]}$$

for $n \ge 1$, see *e.g.*, (1). Eq. **S3** yields

$$\begin{aligned}\binom{N}{\mathbf{n}} &< \frac{N^N\sqrt{2\pi N}}{\prod\limits_{\substack{0\le i<m\\ n_i\neq 0}} n_i^{n_i}\sqrt{2\pi n_i}} \exp\left(\frac{1}{12N} - \sum_{\substack{0\le i<m\\ n_i\neq 0}} \frac{1}{12n_i+1}\right)\\ &< \frac{N^N\sqrt{2\pi N}}{\prod\limits_{\substack{0\le i<m\\ n_i\neq 0}} n_i^{n_i}\sqrt{2\pi n_i}}\end{aligned} \qquad \textbf{[S4]}$$

where the second inequality holds if at least two of $n_0, \ldots, n_{m-1}$ are nonzero. If this is not the case, both sides of Eq. **S2** are equal to 1.

**Expressing $\langle C_L\rangle_N$ in Terms of $\langle \Omega_L\rangle_N$.** Consider a given network, and let $\mathcal{C}_L$ denote the set of states, $\mathbf{Q}$, that represents a proper $L$-cycle of the network. Let $\omega_L$ denote the non-proper counterpart to $\mathcal{C}_L$, meaning that $\omega_L = \bigcup_{\ell|L} \mathcal{C}_L$ where $\ell|L$ means that $\ell$ divides $L$. Then

$$\mathcal{C}_L = \omega_L \setminus \bigcup_{\substack{1\le \ell<L\\ \ell|L}} \omega_\ell = \omega_L \setminus \bigcup_{\substack{d \text{ prime}\\ d|L}} \omega_{L/d} \qquad \textbf{[S5]}$$

since any positive $\ell$ dividing $L$ is also a divisor to a number of the form $L/d$ where $d$ is a prime.

Let $\Omega_L$ denote the number of elements in $\omega_L$. Then, the set theoretic principle of inclusion–exclusion, applied to **S5**, yields

$$LC_L = \sum_{\mathbf{s}\in\{0,1\}^{\eta_L}} (-1)^s \Omega_{L/d_L(\mathbf{s})} \qquad \textbf{[S6]}$$

where $s = \sum_{i=1}^{\eta_L} s_i$, $d_L(\mathbf{s}) = \prod_{i=1}^{\eta_L} (d_L^i)^{s_i}$ and $d_L^1, \ldots, d_L^{\eta_L}$ are the prime divisors to $L$. For averages over randomly chosen $N$-node networks, we get

$$\langle C_L \rangle_N = \frac{1}{L} \sum_{\mathbf{s}\in\{0,1\}^{\eta_L}} (-1)^s \langle \Omega_{L/d_L(\mathbf{s})} \rangle_N \ . \qquad \textbf{[S7]}$$

$\langle \Omega_L \rangle_N$ is given by

$$\langle \Omega_L \rangle_N = \sum_{\substack{\mathbf{n}\in\mathbb{N}^m \\ n=N}} \binom{N}{\mathbf{n}} P_L^N(\mathbf{Q}) \qquad \textbf{[S8]}$$

where $n = n_0 + \cdots + n_{m-1}$. Now, the summation can be split into

$$\langle \Omega_L \rangle_N = \sum_{\hat{\mathbf{n}}\in\mathbb{N}^{m-2}} \sum_{\substack{n_0,n_1\in\mathbb{N} \\ n=N}} \binom{N}{\mathbf{n}} P_L^N(\mathbf{Q}) \qquad \textbf{[S9]}$$

where $\hat{\mathbf{n}} = (n_2, \ldots, n_{m-1})$.

**Calculation of the Inner Sum in the Expression for $\langle \Omega_L \rangle_\infty$.** Let

$$B_L^N(\hat{\mathbf{n}}) = \sum_{\substack{n_0,n_1\in\mathbb{N} \\ n=N}} \binom{N}{\mathbf{n}} P_L^N(\mathbf{Q}) \ . \qquad \textbf{[S10]}$$

Then,

$$\langle \Omega_L \rangle_N = \sum_{\hat{\mathbf{n}}\in\mathbb{N}^{m-2}} B_L^N(\hat{\mathbf{n}}) \qquad \textbf{[S11]}$$

where

$$B_L^N(\hat{\mathbf{n}}) = N! \sum_{\substack{n_0,n_1\in\mathbb{N} \\ n=N}} \prod_{\substack{0\le i<m \\ n_i\neq 0}} \frac{[A_L^i(\mathbf{n}/N)]^{n_i}}{n_i!} \ . \qquad \textbf{[S12]}$$

To calculate $B_L^\infty(\hat{\mathbf{n}}) \equiv \lim_{N\to\infty} B_L^N(\hat{\mathbf{n}})$, we apply Stirling's formula to $N!$, $n_0!$ and $n_1!$ which yields

$$B_L^N(\hat{\mathbf{n}}) \approx \frac{\sqrt{N} N^N}{\sqrt{2\pi} e^{\hat{n}}} \sum_{\substack{0<n_0,n_1 \\ n=N}} \frac{[A_L^0(\mathbf{n}/N)]^{n_0}}{\sqrt{n_0} n_0^{n_0}} \frac{[A_L^1(\mathbf{n}/N)]^{n_1}}{\sqrt{n_1} n_1^{n_1}} \prod_{\substack{2\le i<m \\ n_i\neq 0}} \frac{[A_L^i(\mathbf{n}/N)]^{n_i}}{n_i!} \ . \qquad \textbf{[S13]}$$

where the terms with $n_0 = 0$ or $n_1 = 0$ are ignored. Next, we approximate the sum in Eq. **S13** by an integral, yielding

$$B_L^N(\hat{\mathbf{n}}) \approx \frac{N^{\hat{n}}}{e^{\hat{n}}} \sqrt{\frac{N}{2\pi}} \int_{\substack{0<x_0,x_1 \\ x_0+x_1+\hat{x}=1}} dx_0 \, \frac{e^{N\hat{f}_L(\mathbf{x})}}{\sqrt{x_0 x_1}} \qquad \textbf{[S14]}$$

where $\hat{n} = n_2 + \cdots + n_{m-1}$, $\mathbf{x} = \mathbf{n}/N$, $\hat{x} = \hat{n}/N$ and

$$\hat{f}_L(\mathbf{x}) = x_0 \ln \frac{A_L^0(\mathbf{x})}{x_0} + x_1 \ln \frac{A_L^1(\mathbf{x})}{x_1} + \sum_{\substack{2 \le i < m \\ n_i \neq 0}} x_i \ln A_L^i(\mathbf{x}) - \sum_{i=2}^{m-1} \ln n_i! \ . \qquad \textbf{[S15]}$$

Since the only solution to Eq. **22** (given that $r < 1$) is $x_0 = w_{\mathrm{eq}}$, $x_1 = 1 - w_{\mathrm{eq}}$ and $x_i = 0$ for $i = 2, \ldots, m-1$, we can find the asymptotic behavior of $B_L^\infty$ by a Taylor expansion around this point. Let $x_0 = w_{\mathrm{eq}}(1-\hat{x}) + \epsilon$, $x_1 = (1 - w_{\mathrm{eq}})(1-\hat{x}) - \epsilon$ and $x_i = \hat{x} n_i/\hat{n}$ for $i = 2, \ldots, m-1$. Then,

$$A_L^0(\mathbf{x}) = w_{\mathrm{eq}}(1 - r\hat{x}) + \Delta r\epsilon + a\epsilon^2 + \mathcal{O}(\hat{x}^2) + \mathcal{O}(\hat{x}\epsilon) + \mathcal{O}(\epsilon^3) \qquad \textbf{[S16]}$$

$$A_L^1(\mathbf{x}) = (1 - w_{\mathrm{eq}})(1 - r\hat{x}) - \Delta r\epsilon - a\epsilon^2 + \mathcal{O}(\hat{x}^2) + \mathcal{O}(\hat{x}\epsilon) + \mathcal{O}(\epsilon^3) \qquad \textbf{[S17]}$$

and

$$A_L^i(\mathbf{x}) = \hat{\mathbf{x}} \cdot \nabla A_L^i + \mathcal{O}(\hat{x}^2) + \mathcal{O}(\hat{x}\epsilon) \qquad \textbf{[S18]}$$

for $i = 2, \ldots, m-1$ where $a$ is a constant. Here, $\mathcal{O}(\hat{x}^i\epsilon^j)$ stands for an arbitrary function such that the limit of $\mathcal{O}(\hat{x}^i\epsilon^j)/(\hat{x}^i\epsilon^j)$ is well defined as $(\hat{x}, \epsilon) \to (0, 0)$.

A Taylor expansion of Eq. **S15** yields

$$\begin{aligned} \hat{f}_L(\mathbf{x}) = (1-r)\hat{x} - \frac{(1-r)^2}{w_{\mathrm{eq}}(1-w_{\mathrm{eq}})}\epsilon^2 + \hat{x} \sum_{\substack{2 \le i < m \\ n_i \neq 0}} \frac{n_i}{\hat{n}} \ln \hat{x} \cdot \nabla A_L^i - \sum_{i=2}^{m-1} \ln n_i! \\ + \mathcal{O}(\hat{x}^2) + \mathcal{O}(\hat{x}\epsilon) + \mathcal{O}(\epsilon^3) \ . \end{aligned} \qquad \textbf{[S19]}$$

Completion of the square in Eq. **S19** yields

$$\begin{aligned} \hat{f}_L(\mathbf{x}) = -\frac{1}{2}\left(\frac{1-r}{\sqrt{w_{\mathrm{eq}}(1-w_{\mathrm{eq}})}}\epsilon + \mathcal{O}(\hat{x})\right)^2 + (1-r)\hat{x} + \hat{x} \sum_{\substack{2 \le i < m \\ n_i \neq 0}} \frac{n_i}{\hat{n}} \ln \hat{x} \cdot \nabla A_L^i \\ - \sum_{i=2}^{m-1} \ln n_i! + \mathcal{O}(\hat{x}^2) + \mathcal{O}(\hat{x}\epsilon^2) + \mathcal{O}(\epsilon^3) \ . \end{aligned} \qquad \textbf{[S20]}$$

Now, we can apply the saddle point approximation to Eq. **S14** (given that $r < 1$) together with the relation $\hat{x} = \hat{n}/N$, the convergence of Stirling's formula, and the convergence of the integral approximation. This yields

$$B_L^\infty(\hat{\mathbf{n}}) = \frac{1}{1 - \Delta r} e^{-r\hat{n}} \prod_{\substack{2 \le i < m \\ n_i \neq 0}} \frac{(\hat{\mathbf{n}} \cdot \nabla A_L^i)^{n_i}}{n_i!} \ . \qquad \textbf{[S21]}$$

**Calculation of $g_\ell^\pm$.** With implicit summation over indices occurring both up and down, Eq. **25** can be written as

$$g_\ell^+ = G^{\nu_{\ell-1}^+\nu_{\ell-1}^-}_{\nu_\ell^+\nu_\ell^-} G^{\nu_{\ell-2}^+\nu_{\ell-2}^-}_{\nu_{\ell-1}^+\nu_{\ell-1}^-} \cdots G^{\nu_1^+\nu_1^-}_{\nu_2^+\nu_2^-} G^{\nu_\ell^+\nu_\ell^-}_{\nu_1^+\nu_1^-} \equiv \mathrm{Tr}(\mathbf{G}^\ell) \qquad \textbf{[S22]}$$

$$g_\ell^- = S^{\nu_\ell^+\nu_\ell^-}_{\nu_0^+\nu_0^-} G^{\nu_{\ell-1}^+\nu_{\ell-1}^-}_{\nu_\ell^+\nu_\ell^-} G^{\nu_{\ell-2}^+\nu_{\ell-2}^-}_{\nu_{\ell-1}^+\nu_{\ell-1}^-} \cdots G^{\nu_1^+\nu_1^-}_{\nu_2^+\nu_2^-} G^{\nu_0^+\nu_0^-}_{\nu_1^+\nu_1^-} \equiv \mathrm{Tr}(\mathbf{S}\mathbf{G}^\ell) \qquad \textbf{[S23]}$$

where

$$S^{\mu^+\mu^-}_{\nu^+\nu^-} \equiv \delta_{\nu^+\mu^-}\delta_{\nu^-\mu^+} \qquad \textbf{[S24]}$$

and the trace operator is defined as

$$\mathrm{Tr}(\mathbf{A}) \equiv A^{\nu^+\nu^-}_{\nu^+\nu^-} \; . \qquad \textbf{[S25]}$$

$\delta$ denotes the Kronecker-delta, meaning that $\delta_{\nu\mu} = 1$ if $\nu = \mu$ and 0 otherwise.

By transforming $\mathbf{G}$ in a suitable way, $g_\ell^\pm$ can be calculated in a closed form. Central to this transformation are the tensors $\mathbf{M}$ and $\widetilde{\mathbf{M}}$ that extract moments and combinatorial moments according to the definitions

$$M^{\mu^+\mu^-}_{\kappa^+\kappa^-} \equiv (\mu^+)^{\kappa^+}(\mu^-)^{\kappa^-} \qquad \textbf{[S26]}$$

and

$$\widetilde{M}^{\mu^+\mu^-}_{\kappa^+\kappa^-} \equiv \mu^+(\mu^+ - 1)\cdots(\mu^+ - \kappa^+ + 1)\mu^-(\mu^- - 1)\cdots(\mu^- - \kappa^- + 1) \; . \qquad \textbf{[S27]}$$

Eq. **S26** is interpreted with the convention that $0^0 = 1$ to handle the cases where $\mu^+ = \kappa^+ = 0$ or $\mu^- = \kappa^- = 0$. Henceforth, this convention is used to handle similar special cases conveniently. $\widetilde{\mathbf{M}}$ is triangular in the sense that $\kappa^+ \le \mu^+$ and $\kappa^- \le \mu^-$ for all non-zero elements $\widetilde{M}^{\mu^+\mu^-}_{\kappa^+\kappa^-}$. Hence, $\widetilde{\mathbf{M}}$ has an inverse that obeys $\mu^+ \le \kappa^+$ and $\mu^- \le \kappa^-$ for all non-zero elements $(\widetilde{M}^{-1})^{\kappa^+\kappa^-}_{\mu^+\mu^-}$.

Letting $\widetilde{\mathbf{M}}$ act on $\mathbf{G}$ yields

$$\widetilde{M}^{\mu^+\mu^-}_{\kappa^+\kappa^-} G^{\nu^+\nu^-}_{\mu^+\mu^-} = \sum_{\mu^+=\kappa^+}^{\infty} \sum_{\mu^-=\kappa^-}^{\infty} \exp(-\tilde{\nu}^+)\frac{(\tilde{\nu}^+)^{\mu^+}}{(\mu^+ - \kappa^+)!} \exp(-\tilde{\nu}^-)\frac{(\tilde{\nu}^-)^{\mu^-}}{(\mu^- - \kappa^-)!} \qquad \textbf{[S28]}$$

$$= (\tilde{\nu}^+)^{\kappa^+}(\tilde{\nu}^-)^{\kappa^-} \qquad \textbf{[S29]}$$

where $\tilde{\nu}^\pm \equiv r^{\mathrm{C}}\nu^\pm + r^{\mathrm{I}}\nu^\mp$.

Let $C^{\kappa^+\kappa^-}_{\lambda^+\lambda^-}$ denote the coefficients of the formal expansion of $(z^+ + z^-)^{\lambda^+}(z^+ - z^-)^{\lambda^-}$ in such a way that

$$(z^+ + z^-)^{\lambda^+}(z^+ - z^-)^{\lambda^-} \equiv \sum_{\kappa^+,\kappa^- \in \mathbb{N}} C^{\kappa^+\kappa^-}_{\lambda^+\lambda^-}(z^+)^{\kappa^+}(z^-)^{\kappa^-} \; . \qquad \textbf{[S30]}$$

Note that $\mathbf{C}$ is block diagonal in the sense that $\kappa^+ + \kappa^- = \lambda^+ + \lambda^-$ for all non-zero elements. The inverse of $\mathbf{C}$ is given by

$$(C^{-1})^{\lambda^+\lambda^-}_{\kappa^+\kappa^-} = 2^{-\kappa^+-\kappa^-} C^{\lambda^+\lambda^-}_{\kappa^+\kappa^-} \; . \qquad \textbf{[S31]}$$

To see this, we consider that $\mathbf{C}^2$ yields the coefficients of the formal expansion of the expression

$$[(z^+ + z^-) + (z^+ - z^-)]^{\lambda^+}[(z^+ + z^-) - (z^+ - z^-)]^{\lambda^-} \equiv 2^{\lambda^+ + \lambda^-}(z^+)^{\lambda^+}(z^-)^{\lambda^-} \ . \tag{S32}$$

Thus,

$$C^{\kappa^+\kappa^-}_{\lambda^+\lambda^-} C^{\nu^+\nu^-}_{\kappa^+\kappa^-} = 2^{\lambda^+ + \lambda^-}\delta_{\lambda^+\nu^+}\delta_{\lambda^-\nu^-} \tag{S33}$$

which means that the tensor on the left-hand side in Eq. **S31** is the inverse of $\mathbf{C}$.

Letting $\mathbf{C}$ act on $\mathbf{M}$ and $\widetilde{\mathbf{M}}\mathbf{G}$ yields

$$C^{\kappa^+\kappa^-}_{\lambda^+\lambda^-} M^{\mu^+\mu^-}_{\kappa^+\kappa^-} = (\mu^+ + \mu^-)^{\lambda^+}(\mu^+ - \mu^-)^{\lambda^-} \tag{S34}$$

$$C^{\kappa^+\kappa^-}_{\lambda^+\lambda^-} \widetilde{M}^{\mu^+\mu^-}_{\kappa^+\kappa^-} G^{\nu^+\nu^-}_{\mu^+\mu^-} = (\tilde{\nu}^+ + \tilde{\nu}^-)^{\lambda^+}(\tilde{\nu}^+ - \tilde{\nu}^-)^{\lambda^-} \tag{S35}$$

$$= r^{\lambda^+}(\Delta r)^{\lambda^-}(\nu^+ + \nu^-)^{\lambda^+}(\nu^+ - \nu^-)^{\lambda^-} \ . \tag{S36}$$

Hence,

$$\mathbf{C}\widetilde{\mathbf{M}}\mathbf{G} = \mathbf{DCM} \tag{S37}$$

and

$$\mathbf{C}\widetilde{\mathbf{M}}\mathbf{G}\widetilde{\mathbf{M}}^{-1}\mathbf{C}^{-1} = \mathbf{DCM}\widetilde{\mathbf{M}}^{-1}\mathbf{C}^{-1} \tag{S38}$$

where

$$D^{\mu^+\mu^-}_{\lambda^+\lambda^-} \equiv r^{\lambda^+}(\Delta r)^{\lambda^-}\delta_{\lambda^+\mu^+}\delta_{\lambda^-\mu^-} \ . \tag{S39}$$

Since $\widetilde{\mathbf{M}}^{-1}$ is triangular with the lower indices (acting to the left) less than or equal to the upper indices, right multiplication with $\widetilde{\mathbf{M}}^{-1}$ yields always a convergent result. Similarly, $\mathbf{C}^{-1}$ is well-behaved in the same sense, as a consequence of the block diagonal structure of $\mathbf{C}$. Thus, both sides of the equality in Eq. **S38** are well-defined.

Let $\mathbf{T} = \mathbf{CM}\widetilde{\mathbf{M}}^{-1}\mathbf{C}^{-1}$, which yields

$$\mathbf{C}\widetilde{\mathbf{M}}\mathbf{G}\widetilde{\mathbf{M}}^{-1}\mathbf{C}^{-1} = \mathbf{DT} \ . \tag{S40}$$

The tensor $\mathbf{M}\widetilde{\mathbf{M}}^{-1}$ tells how to express moments in terms of combinatorial moments. Each moment can be expressed as a sum of the combinatorial moment of the same order and a linear combination of combinatorial moments of lower order. Hence,

$$M^{\mu^+\mu^-}_{\kappa^+\kappa^-}(\widetilde{M}^{-1})^{\lambda^+\lambda^-}_{\mu^+\mu^-} = \delta_{\kappa^+\lambda^+}\delta_{\kappa^-\lambda^-} \qquad \text{for } \lambda^+ + \lambda^- \geq \kappa^+ + \kappa^-. \tag{S41}$$

This property is conserved as $\mathbf{M}\widetilde{\mathbf{M}}^{-1}$ is transformed by $\mathbf{C}$, since

$$C^{\kappa^+\kappa^-}_{\nu^+\nu^-} = 0 \qquad \text{for } \kappa^+ + \kappa^- \neq \nu^+ + \nu^- \ , \tag{S42}$$

meaning that

$$T^{\mu^+\mu^-}_{\nu^+\nu^-} = \delta_{\nu^+\mu^+}\delta_{\nu^-\mu^-} \qquad \text{for } \mu^+ + \mu^- \geq \nu^+ + \nu^- \ . \tag{S43}$$

Eq. **S22** can be rewritten as

$$g_\ell^+ = \mathrm{Tr}(\mathbf{G}^\ell) = \mathrm{Tr}\big[(\mathbf{C}\widetilde{\mathbf{M}}\mathbf{G}\widetilde{\mathbf{M}}^{-1}\mathbf{C}^{-1})^\ell\big] = \mathrm{Tr}\big[(\mathbf{D}\mathbf{T})^\ell\big] \ . \tag{S44}$$

In order to treat Eq. **S23** similarly, we need to transform **GS** in the same manner. To do this, we observe that

$$\begin{aligned}(C\widetilde{M}G)^{\mu^+\mu^-}_{\lambda^+\lambda^-} S^{\nu^+\nu^-}_{\mu^+\mu^-} &= r^{\lambda^+}(\Delta r)^{\lambda^-}(\nu^- + \nu^+)^{\lambda^+}(\nu^- - \nu^+)^{\lambda^-} &\text{[S45]}\\ &= r^{\lambda^+}(-\Delta r)^{\lambda^-}(\nu^+ + \nu^-)^{\lambda^+}(\nu^+ - \nu^-)^{\lambda^-} \ , &\text{[S46]}\end{aligned}$$

which means that

$$\mathbf{C}\widetilde{\mathbf{M}}\mathbf{G}\mathbf{S} = \acute{\mathbf{S}}\mathbf{C}\widetilde{\mathbf{M}}\mathbf{G} \tag{S47}$$

where

$$\acute{S}^{\kappa^+\kappa^-}_{\lambda^+\lambda^-} \equiv (-1)^{\lambda^-}\delta_{\lambda^+\kappa^+}\delta_{\lambda^-\kappa^-} \ . \tag{S48}$$

Hence,

$$\mathbf{C}\widetilde{\mathbf{M}}\mathbf{G}\mathbf{S}\widetilde{\mathbf{M}}^{-1}\mathbf{C}^{-1} = \acute{\mathbf{S}}\mathbf{D}\mathbf{T} \tag{S49}$$

which can be applied to Eq. **S23**, yielding

$$g_\ell^- = \mathrm{Tr}(\mathbf{S}\mathbf{G}^\ell) = \mathrm{Tr}\big[\mathbf{C}\widetilde{\mathbf{M}}\mathbf{G}\mathbf{S}\widetilde{\mathbf{M}}^{-1}\mathbf{C}^{-1}(\mathbf{C}\widetilde{\mathbf{M}}\mathbf{G}\widetilde{\mathbf{M}}^{-1}\mathbf{C}^{-1})^{\ell-1}\big] = \mathrm{Tr}\big[\acute{\mathbf{S}}(\mathbf{T}\mathbf{D})^\ell\big] \ . \tag{S50}$$

Since **T** is triangular with unitary diagonal, according to Eq. **S43**, while $\acute{\mathbf{S}}$ and **D** are diagonal, the traces in Eqs. **S44** and **S50** are given by

$$\begin{aligned} g_\ell^+ &= \mathrm{Tr}\big[(\mathbf{T}\mathbf{D})^\ell\big] &\text{[S51]}\\ &= \big(D^{\mu^+\mu^-}_{\mu^+\mu^-}\big)^\ell &\text{[S52]}\\ &= \sum_{\mu^+,\mu^-\in\mathbb{N}} r^{\ell\mu^+}(\Delta r)^{\ell\mu^-} &\text{[S53]}\\ &= \frac{1}{1-r^\ell}\frac{1}{1-(\Delta r)^\ell} &\text{[S54]}\end{aligned}$$

and

$$\begin{aligned} g_\ell^- &= \mathrm{Tr}\big[\acute{\mathbf{S}}(\mathbf{T}\mathbf{D})^\ell\big] &\text{[S55]}\\ &= \acute{S}^{\mu^+\mu^-}_{\mu^+\mu^-}\big(D^{\mu^+\mu^-}_{\mu^+\mu^-}\big)^\ell &\text{[S56]}\\ &= \sum_{\mu^+,\mu^-\in\mathbb{N}} (-1)^{\mu^-} r^{\ell\mu^+}(\Delta r)^{\ell\mu^-} &\text{[S57]}\\ &= \frac{1}{1-r^\ell}\frac{1}{1+(\Delta r)^\ell} \ . &\text{[S58]}\end{aligned}$$

Finally, we conclude that

$$g_\ell^\pm = \frac{1}{1-r^\ell}\frac{1}{1\mp(\Delta r)^\ell} \ . \tag{S59}$$

**Calculation of $\langle \Omega_L \rangle_\infty$.** In order to use Eq. **29** to calculate $\langle \Omega_L \rangle_\infty$, we need to find the distribution of lengths and parities of the invariant sets of $L$-cycles series. For $L$-cycles, there will be invariant sets of length $\ell$ and positive parity if $\ell | L$, while sets of negative parity are present if $2\ell | L$. The number of invariant sets with a specific length and parity is independent of $L$ (as long as they exist at all) since the basic form of the series in such sets does not change with $L$. Only the number of basic repetitions alter. Let $J_\ell^+$ and $J_\ell^-$ denote the numbers of invariant sets of length $\ell$ with positive or negative parity respectively.

Let $\psi_\ell^+$ respective $\psi_\ell^-$ denote the sets of (infinite) time series of 'true' and 'false' such that each series is identical to, or the inverse of, itself after $\ell$ time steps. Then, the set of time series that are part of an invariant set of $L$-cycles with length $\ell$ and negative parity, $\mathcal{J}_\ell^-$, is given by

$$\mathcal{J}_\ell^- = \psi_\ell^- \setminus \bigcup_{\substack{d \text{ odd prime} \\ d|\ell}} \psi_{\ell/d}^- \, . \quad \textbf{[S60]}$$

For positive parity, we get

$$\mathcal{J}_\ell^+ = \psi_\ell^+ \Bigg\backslash \left( \bigcup_{\substack{d \text{ prime} \\ d|\ell}} \psi_{\ell/d}^+ \right) \Bigg\backslash \mathcal{J}_{\ell/2}^- \quad \textbf{[S61]}$$

where $\mathcal{J}_{\ell/2}^-$ is the empty set if $\ell/2$ is not an integer.

The numbers of elements in $\mathcal{J}_\ell^\pm$ are given by $2\ell J_\ell^\pm$ where $J_\ell^\pm$ are the numbers of invariant sets with length $\ell$. Then, the inclusion–exclusion principle yields

$$J_\ell^- = \frac{1}{2\ell} \sum_{\mathbf{s} \in \{0,1\}^{\tilde{\eta}_\ell}} (-1)^s 2^{\ell/\tilde{d}_\ell(\mathbf{s})} \quad \textbf{[S62]}$$

where $s = \sum_{i=1}^{\tilde{\eta}_\ell} s_i$, $\tilde{d}(\mathbf{s}) = \prod_{i=1}^{\tilde{\eta}_\ell} (\tilde{d}_\ell^i)^{s_i}$ and $\tilde{d}_\ell^1, \ldots, \tilde{d}_\ell^{\eta_\ell}$ are the odd prime divisors to $\ell$. Similarly

$$J_\ell^+ = \frac{1}{2\ell} \sum_{\substack{s_0 \in \{0,1\} \\ 2^{s_0} | \ell}} \sum_{\mathbf{s} \in \{0,1\}^{\tilde{\eta}_\ell}} (-1)^{s_0 + s} 2^{\ell/d_\ell(s_0, \mathbf{s})} - \frac{1}{2} J_{\ell/2}^- \quad \textbf{[S63]}$$

where $d(s_0, \mathbf{s}) = 2^{s_0} \tilde{d}(\mathbf{s})$ and $J_{\ell/2}^- = 0$ if $\ell/2$ is not an integer. Insertion of Eq. **S62** into Eq. **S63** yields

$$J_\ell^+ = \frac{1}{2\ell} \sum_{\substack{s_0 \in \{0,1\} \\ 2^{s_0} | \ell}} \sum_{\mathbf{s} \in \{0,1\}^{\tilde{\eta}_\ell}} (1 + s_0)(-1)^{s_0 + s} 2^{\ell/d_\ell(s_0, \mathbf{s})} \quad \textbf{[S64]}$$

which also can be written as

$$J_\ell^+ = J_\ell^- - J_{\ell/2}^- \, . \quad \textbf{[S65]}$$

Finally, we can calculate $\langle\Omega_L\rangle_\infty$ according to

$$\langle\Omega_L\rangle_\infty = (1-r)\prod_{\ell|L}(g_\ell^+)^{J_\ell^+}\prod_{2\ell|L}(g_\ell^-)^{J_\ell^-} \; . \qquad \textbf{[S66]}$$

The factor $(1-r)$ instead of $1/(1-\Delta r)$ is there to compensate for the factor $g(\rho_L^0) = g_1^+$, which is not included in Eq. **29**.

**Convergence of $\langle C\rangle_\infty$.** For large $\ell$, we can use the approximations

$$\ln g_\ell^\pm = -\ln(1-r^\ell) - \ln[1\mp(\Delta r)^\ell] \approx r^\ell \pm (\Delta r)^\ell \qquad \textbf{[S67]}$$

and

$$J_\ell^\pm = \frac{2^\ell}{2\ell} \qquad \textbf{[S68]}$$

with relative error that decreases exponentially with $\ell$. Thus, the correct asymptotic behavior of $\langle\Omega_L\rangle_\infty$ is revealed by

$$\langle\Omega_L\rangle_\infty \sim \exp\left\{\sum_{\ell|L}\frac{2^\ell}{2\ell}\left[r^\ell+(\Delta r)^\ell\right]+\sum_{2\ell|L}\frac{2^\ell}{2\ell}\left[r^\ell-(\Delta r)^\ell\right]\right\} \; . \qquad \textbf{[S69]}$$

If $r > 1/2$, Eq. **S69** diverges double exponentially since the term $(2r)^L/(2L)$ will dominate the sum as $L\to\infty$. This means that the number of $L$-cycles increases very rapidly with $L$ for large $L$.

If $r < 1/2$, $|\Delta r| < 1/2$ must hold since $|\Delta r| \le r$. Then, the total number of states in attractors, $\langle\Omega\rangle_\infty$, will converge since Eq. **S69** then yields the convergent sum

$$\langle\Omega\rangle_\infty \sim \exp\sum_{\ell=1}^{\infty}\frac{(2r)^\ell}{\ell} \; . \qquad \textbf{[S70]}$$

Hence, the average of the total number of attractors, $\langle C\rangle_\infty$, will converge for $r < 1/2$ and diverge for $r > 1/2$.

1. Feller, W. (1968) in *An Introduction to Probability Theory and Its Applications, Vol. 1*, 3rd ed. (Wiley, New York), pp. 50-53
